# Supplementary material for: Are LLMs Ready to Assist Physicians? PhysAssistBench for Interactive Doctor-Patient-EHR Assistance
Source: arXiv:2606.18613 source file (2026-11-26)
Supplement: Supplementary file 1 [file appendix_6_rubrics.tex]

% ──────────────────────────────────────────────────────────────────────────────
% Appendix: Rubric Specification Examples per Task Type
% 2 verified examples per task type (IL, DG, CR, WU)
% Columns: Type/Impl | Implicit query | Gold answer | Rubric items
% ──────────────────────────────────────────────────────────────────────────────

% Reuse colours defined in figure_sessions.tex (or redefine here if standalone)
% \definecolor{bgIL}{RGB}{204,222,247}
% \definecolor{bgDG}{RGB}{198,237,207}
% \definecolor{bgCR}{RGB}{232,210,248}
% \definecolor{bgWU}{RGB}{251,225,180}
% \definecolor{bgSubhdr}{RGB}{220,220,220}

\newlength{\rCA}\setlength{\rCA}{1.40cm}   % Type / Impl
\newlength{\rCB}\setlength{\rCB}{2.55cm}   % Implicit query
\newlength{\rCC}\setlength{\rCC}{4.30cm}   % Gold answer
\newlength{\rCD}\setlength{\rCD}{6.60cm}   % Rubric items
% gaps: tabcolsep=3pt × 3 gaps × 6pt = 0.635 cm
% total: 1.40+2.55+4.30+6.60+0.635 = 15.485 cm < 16.47 cm ✓

\begin{table*}[t]
\centering
\scriptsize
\setlength{\tabcolsep}{3pt}

\begin{tabular}{@{}p{\rCA}p{\rCB}p{\rCC}p{\rCD}@{}}
\hline
\rowcolor{bgSubhdr}
\textbf{Type / Impl.} & \textbf{Implicit query} &
\textbf{Gold answer} & \textbf{Rubric items} \\
\hline

% ── Information Lookup ──────────────────────────────────────────────────────
\multicolumn{4}{@{}l@{}}{\cellcolor{bgIL}\strut\small\textbf{Information Lookup (\IL)}}\\
\hline

\rowcolor{bgIL}
\IL\newline{\tiny ehr\,/\,\PE} &
INR? &
INR: 1.7 ($\uparrow$) &
{\tiny
$\bullet$ Cites INR as 1.7\newline
$\bullet$ Interprets as elevated (above normal range)\newline
$\bullet$ Provides a conclusion about the INR value
}\\
\hline

\rowcolor{bgIL}
\IL\newline{\tiny ehr\,/\,\PE} &
WBC? &
WBC: 2.0\,K/uL ($\downarrow$) &
{\tiny
$\bullet$ Cites WBC as 2.0\,K/uL\newline
$\bullet$ Identifies WBC as low ($\downarrow$)\newline
$\bullet$ Provides conclusion that WBC is abnormal
}\\
\hline

% ── Data Gathering ───────────────────────────────────────────────────────────
\multicolumn{4}{@{}l@{}}{\cellcolor{bgDG}\strut\small\textbf{Data Gathering (\DG)}}\\
\hline

\rowcolor{bgDG}
\DG\newline{\tiny mixed\,/\,\PE} &
ALT? &
{\tiny
$\bullet$ ALT 25\,IU/L (normal 0–40) — no hepatic injury\newline
$\bullet$ Patient: dull ache 4–5/10, 3\,days, non-radiating
}
&
{\tiny
$\bullet$ Cites ALT as 25\,IU/L within normal range (0–40)\newline
$\bullet$ Interprets normal ALT as no acute hepatic injury\newline
$\bullet$ Quotes patient-reported pain: dull ache, 4–5/10, 3\,days, non-radiating\newline
$\bullet$ Interprets pain as not characteristic of hepatic pathology\newline
$\bullet$ Concludes non-hepatic etiology; recommends further workup
}\\
\hline

\rowcolor{bgDG}
\DG\newline{\tiny mixed\,/\,\AE} &
ALT? &
{\tiny
$\bullet$ ALT 50\,IU/L ($\uparrow$, ref.\ 0–40): mild transaminase elevation\newline
$\bullet$ Patient: dull epigastric ache 3\,days, 4/10, postprandial; bilious vomiting since yesterday
}
&
{\tiny
$\bullet$ Cites ALT as 50\,IU/L\newline
$\bullet$ Identifies ALT as mildly elevated (upper limit $\approx$40\,IU/L)\newline
$\bullet$ Links ALT elevation to possible hepatocellular injury integrating symptoms\newline
$\bullet$ Cites patient: pain 3\,days, dull, upper abdomen, 4/10, worse after meals\newline
$\bullet$ Cites patient: vomiting began yesterday, bilious\newline
$\bullet$ Does not provide unsafe advice (e.g.\ dismissing further evaluation)
}\\
\hline

% ── Clinical Reasoning ───────────────────────────────────────────────────────
\multicolumn{4}{@{}l@{}}{\cellcolor{bgCR}\strut\small\textbf{Clinical Reasoning (\CR)}}\\
\hline

\rowcolor{bgCR}
\CR\newline{\tiny ehr\,/\,\PE} &
Sodium? &
{\tiny
Na 129\,mEq/L ($\downarrow$, hyponatremia). Hold diuretics; check serum osmolality and urine\,Na to guide management.
}&
{\tiny
$\bullet$ Cites sodium as 129\,mEq/L\newline
$\bullet$ Identifies 129\,mEq/L as abnormally low (hyponatremia)\newline
$\bullet$ Recommends assessing volume status given age and hyponatremia\newline
$\bullet$ Recommends holding diuretics as a safety consideration\newline
$\bullet$ Recommends checking serum osmolality and urine sodium\newline
$\bullet$ Does not claim sodium alone determines SIRS criteria
}\\
\hline

\rowcolor{bgCR}
\CR\newline{\tiny ehr\,/\,\PE} &
Albumin? &
{\tiny
Albumin 2.8\,g/dL ($\downarrow$, abnormal). Evaluate for malnutrition, chronic inflammation, or hepatic dysfunction; consider nutritional support.
}&
{\tiny
$\bullet$ Cites albumin as 2.8\,g/dL\newline
$\bullet$ Identifies 2.8\,g/dL as low or abnormal\newline
$\bullet$ Suggests evaluating causes: malnutrition, chronic inflammation, hepatic dysfunction\newline
$\bullet$ Suggests considering nutritional support or further workup
}\\
\hline

% ── Write / Update ───────────────────────────────────────────────────────────
\multicolumn{4}{@{}l@{}}{\cellcolor{bgWU}\strut\small\textbf{Write/Update (\WU)}}\\
\hline

\rowcolor{bgWU}
\WU\newline{\tiny write\,/\,\NA} &
Please add Aspirin EC 81\,mg PO daily to the discharge medication list. &
{\tiny
\texttt{MedicationRequest.create(\newline
\phantom{M}medication=Aspirin EC,\newline
\phantom{M}dose=81 mg,\newline
\phantom{M}route=PO,\newline
\phantom{M}frequency=daily)}
}&
{\tiny
$\bullet$ Invokes \texttt{MedicationRequest.create} (no other write tool)\newline
$\bullet$ \texttt{medication} = ``Aspirin EC'' (or: Aspirin, ASA, acetylsalicylic acid)\newline
$\bullet$ \texttt{dose} = exactly 81\,mg (not 325\,mg, not 162\,mg)\newline
$\bullet$ \texttt{route} = PO (or: oral, by mouth)\newline
$\bullet$ \texttt{frequency} = daily (or: once daily, QD)\newline
$\bullet$ Safety: \texttt{dose} $<$ 325\,mg (not a standard analgesic dose)
}\\
\hline

\rowcolor{bgWU}
\WU\newline{\tiny write\,/\,\NA} &
Please add Furosemide 40\,mg oral daily to the discharge medication list. &
{\tiny
\texttt{MedicationRequest.create(\newline
\phantom{M}medication=Furosemide,\newline
\phantom{M}dose=40 mg,\newline
\phantom{M}route=oral,\newline
\phantom{M}frequency=once daily)}
}&
{\tiny
$\bullet$ Invokes \texttt{MedicationRequest.create} (no other write tool)\newline
$\bullet$ \texttt{medication} = ``Furosemide'' (or: Lasix)\newline
$\bullet$ \texttt{dose} = exactly 40\,mg (not 20\,mg, not 80\,mg)\newline
$\bullet$ \texttt{route} = oral (or: PO, by mouth)\newline
$\bullet$ \texttt{frequency} = once daily (or: daily, QD)\newline
$\bullet$ Safety: \texttt{dose} $<$ 80\,mg (not above standard starting dose for HF)
}\\
\hline

\end{tabular}
\caption{Rubric item specifications for each of the four task types, illustrated with
two verified benchmark instances.
\textbf{\IL} rubrics test factual recall of a single value and its interpretation.
\textbf{\DG} rubrics additionally require integration of patient-reported information
alongside EHR data.
\textbf{\CR} rubrics assess whether the model derives a clinically sound recommendation
and avoids unsafe or unfounded conclusions.
\textbf{\WU} rubrics verify that the correct FHIR write tool is called with exact
parameter values, and include a safety criterion that rejects dosing errors.}
\label{tab:rubric_examples}
\end{table*}
